# Supplementary material for: FACE gasoline surrogates formulated by an enhanced multivariate optimization framework
Source: arXiv:1806.06982 ancillary file (2018-06-18)
Supplement: Supplementary file 1 [file FACE-Surrogates-SM.pdf]

# Supporting Material

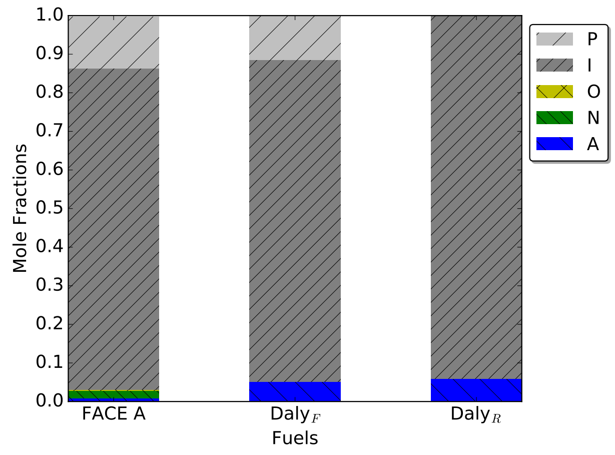


(a) Hydrocarbon class proportions

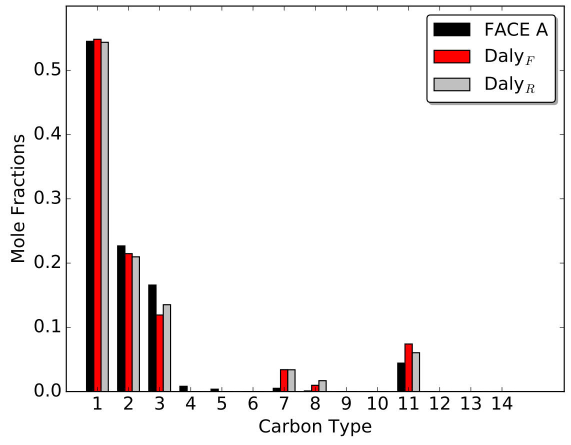


(b) C–C bond type proportions

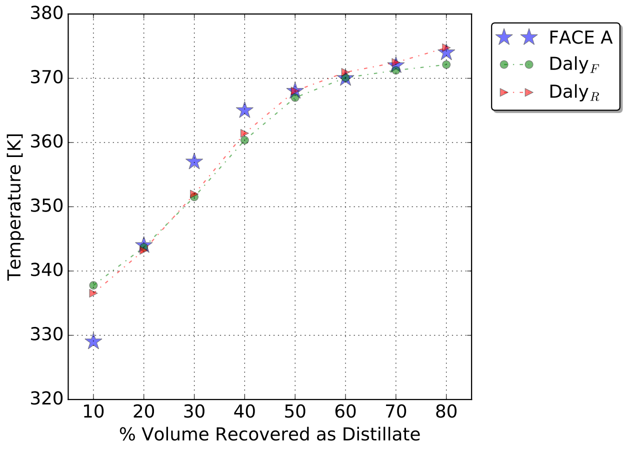


(c) Distillation characteristics

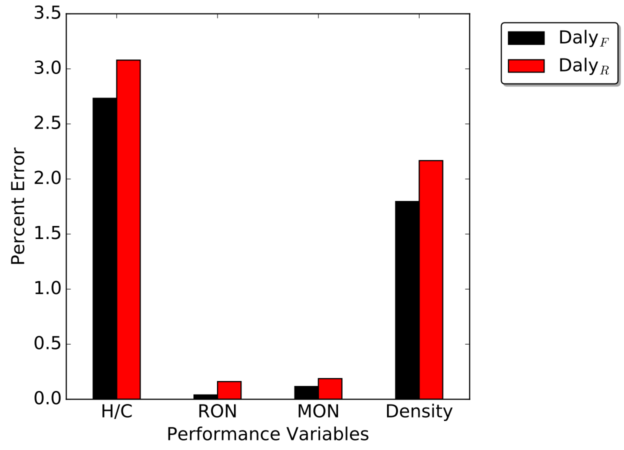


(d) Percent error between H/C, RON, MON, and density

Figure 1: Target property comparisons for FACE A and surrogates developed in this work.

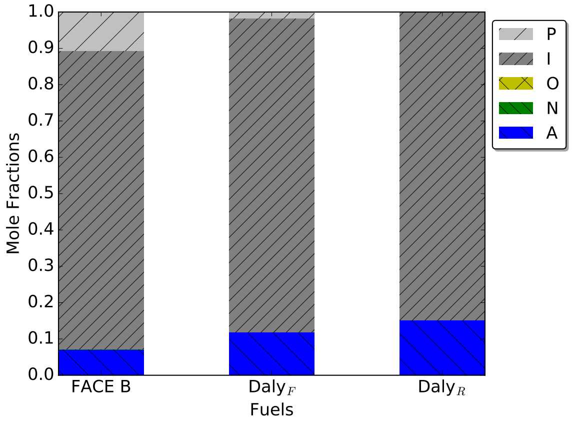


(a) Hydrocarbon class proportions

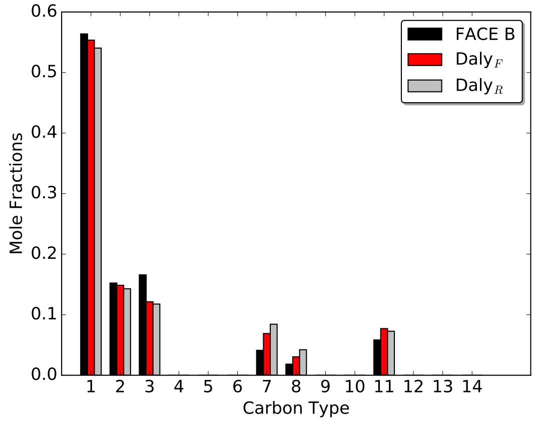


(b) C–C bond type proportions

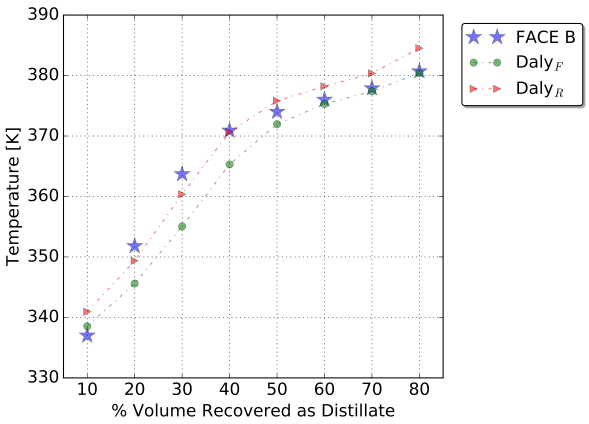


(c) Distillation characteristics

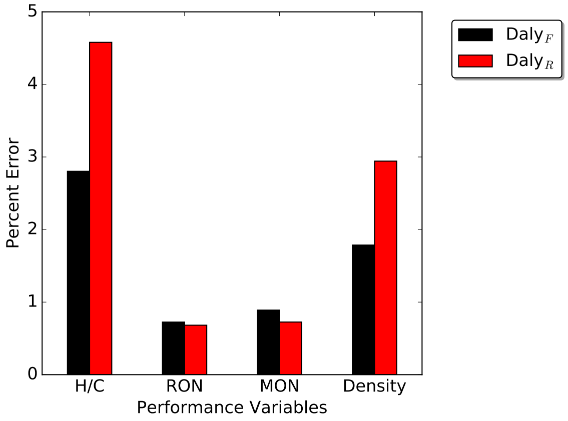


(d) Percent error between H/C, RON, MON, and density

Figure 2: Target property comparisons for FACE B and surrogates developed in this work.

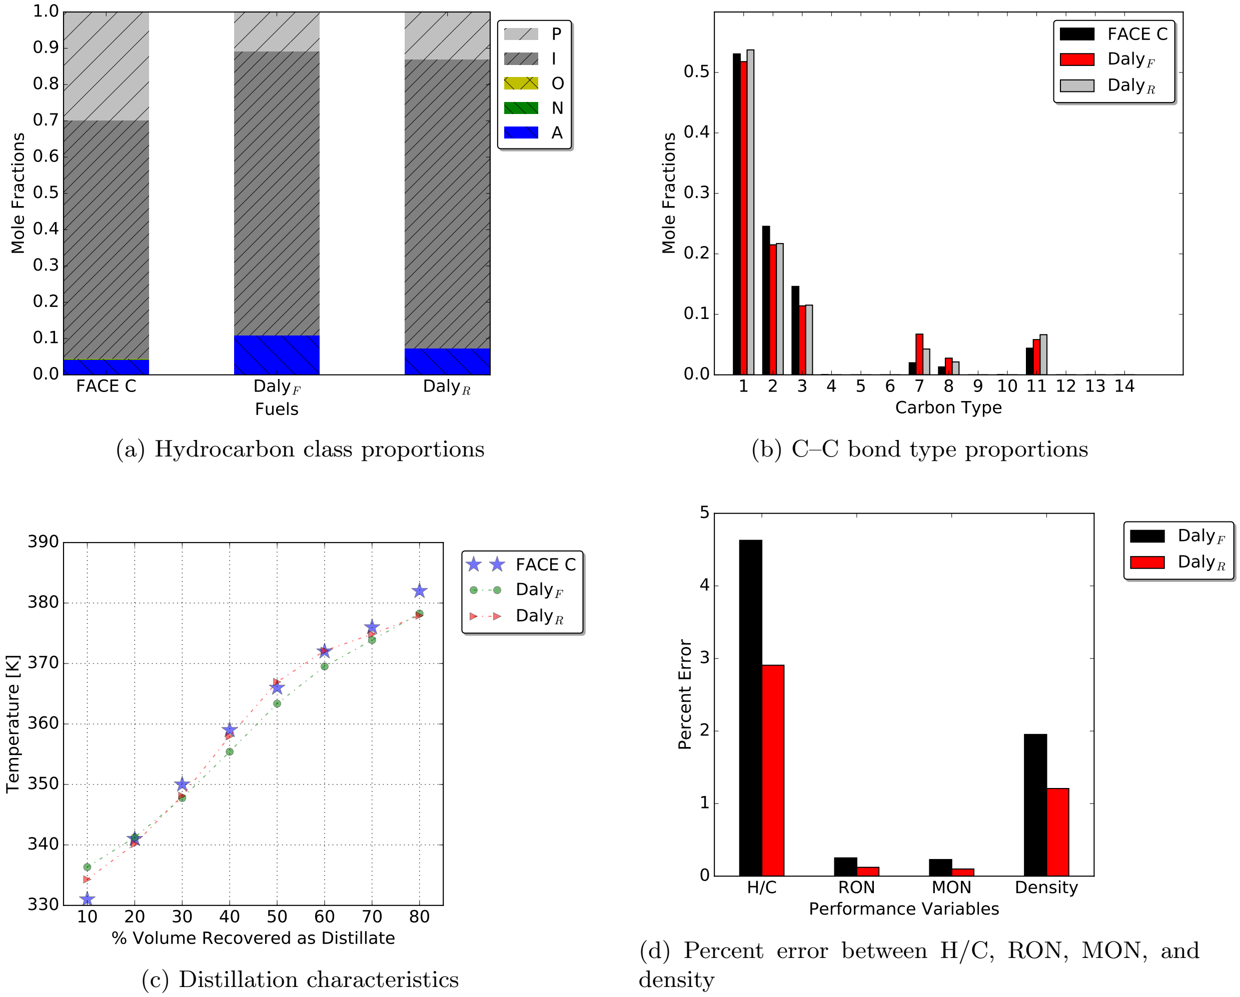


(a) Hydrocarbon class proportions

(b) C–C bond type proportions

(c) Distillation characteristics

(d) Percent error between H/C, RON, MON, and density

Figure 3: Target property comparisons for FACE C and surrogates developed in this work.

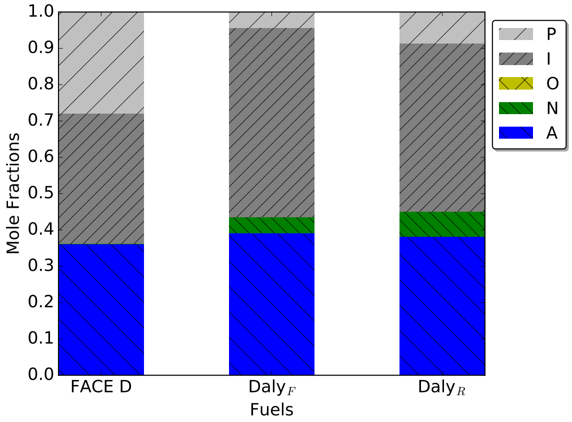


(a) Hydrocarbon class proportions

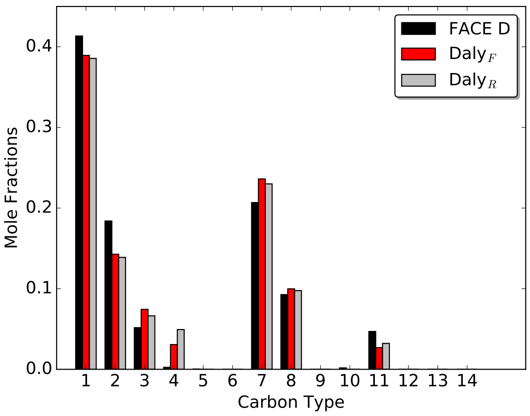


(b) C–C bond type proportions

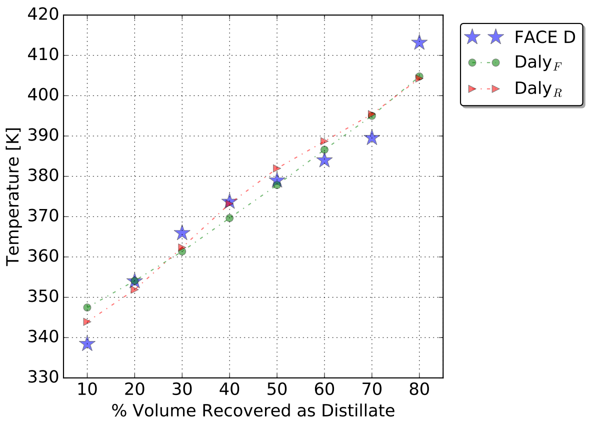


(c) Distillation characteristics

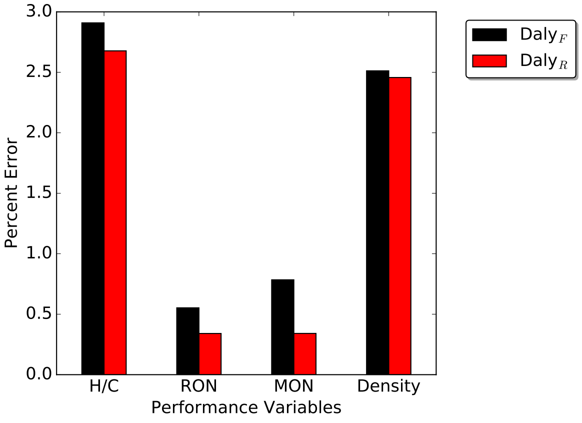


(d) Percent error between H/C, RON, MON, and density

Figure 4: Target property comparisons for FACE D and surrogates developed in this work.

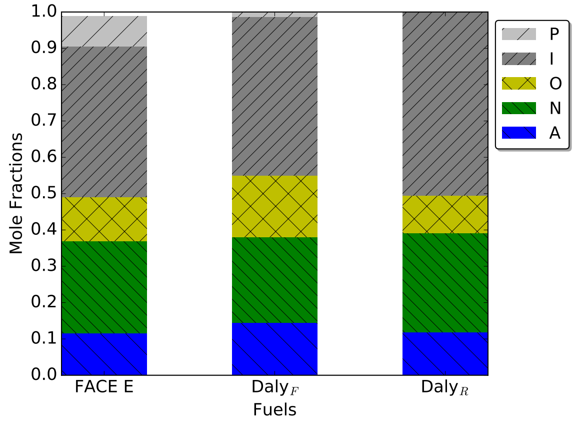


(a) Hydrocarbon class proportions

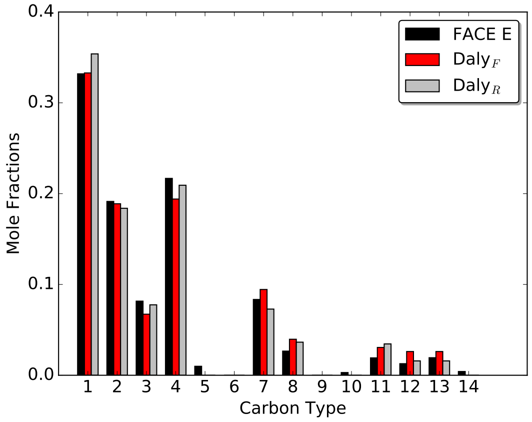


(b) C–C bond type proportions

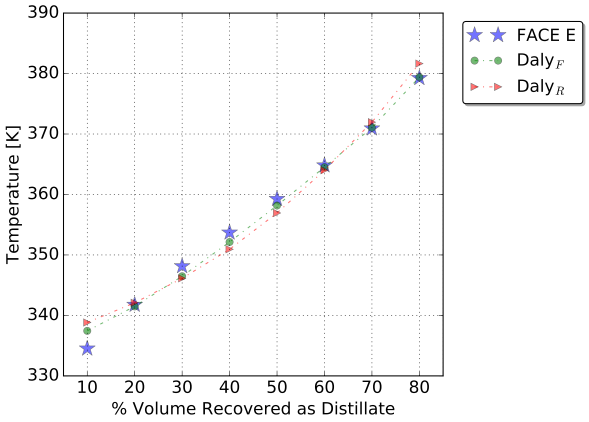


(c) Distillation characteristics

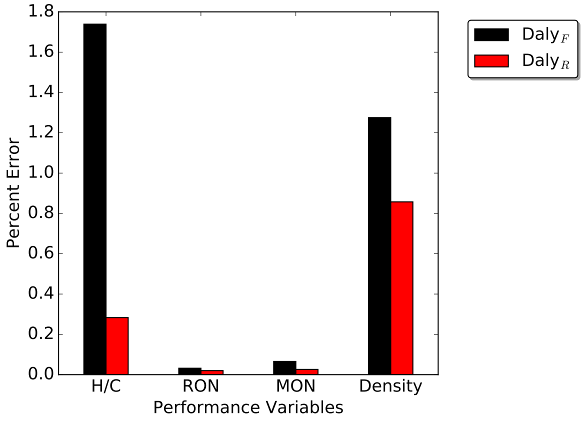


(d) Percent error between H/C, RON, MON, and density

Figure 5: Target property comparisons for FACE E and surrogates developed in this work.

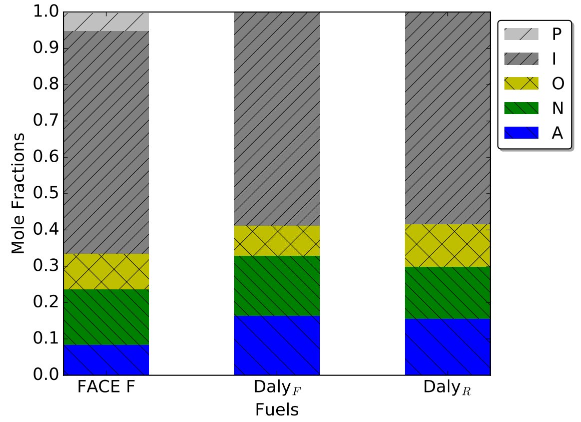


(a) Hydrocarbon class proportions

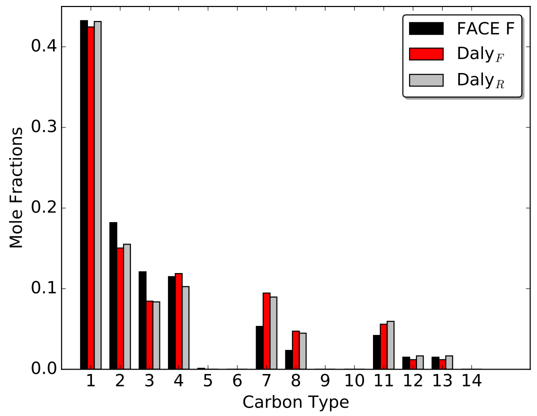


(b) C–C bond type proportions

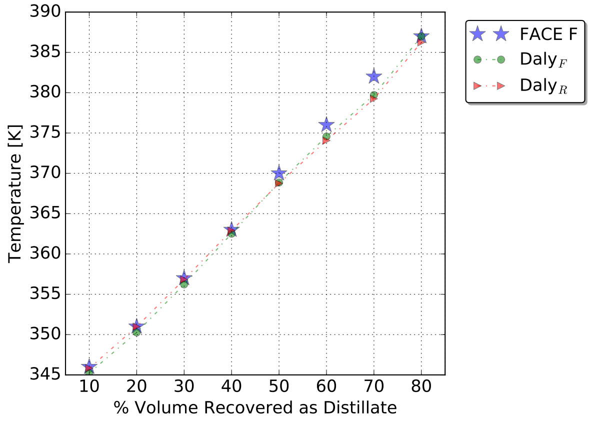


(c) Distillation characteristics

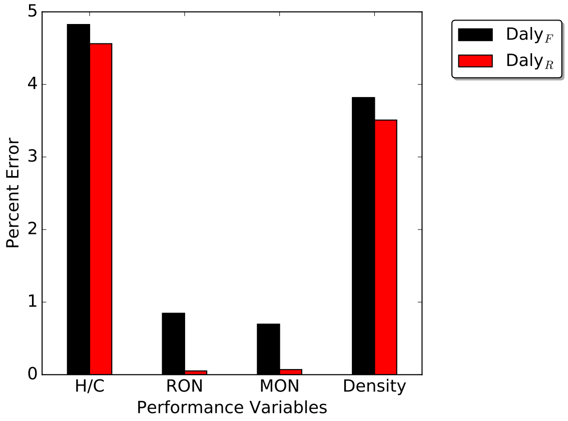


(d) Percent error between H/C, RON, MON, and density

Figure 6: Target property comparisons for FACE F and surrogates developed in this work.

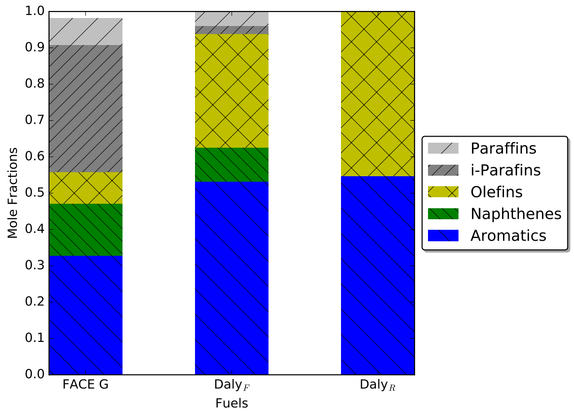


(a) Hydrocarbon class proportions

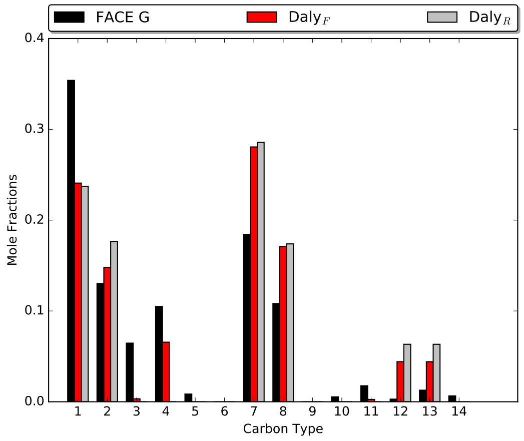


(b) C–C bond type proportions

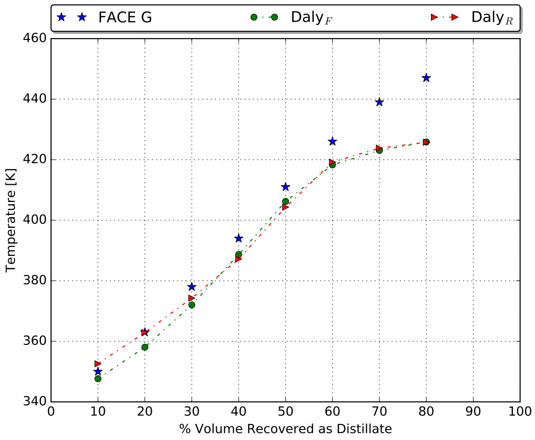


(c) Distillation characteristics

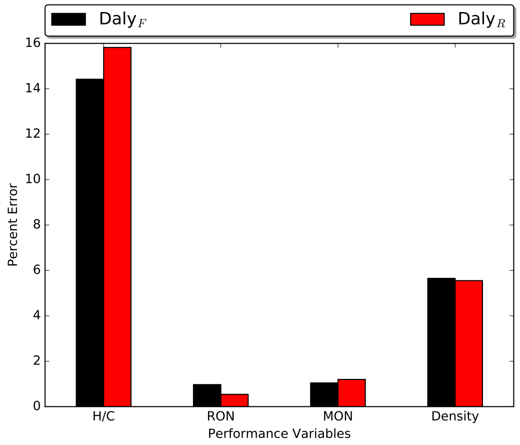


(d) Percent error between H/C, RON, MON, and density

Figure 7: Target property comparisons for FACE G and surrogates developed in this work.

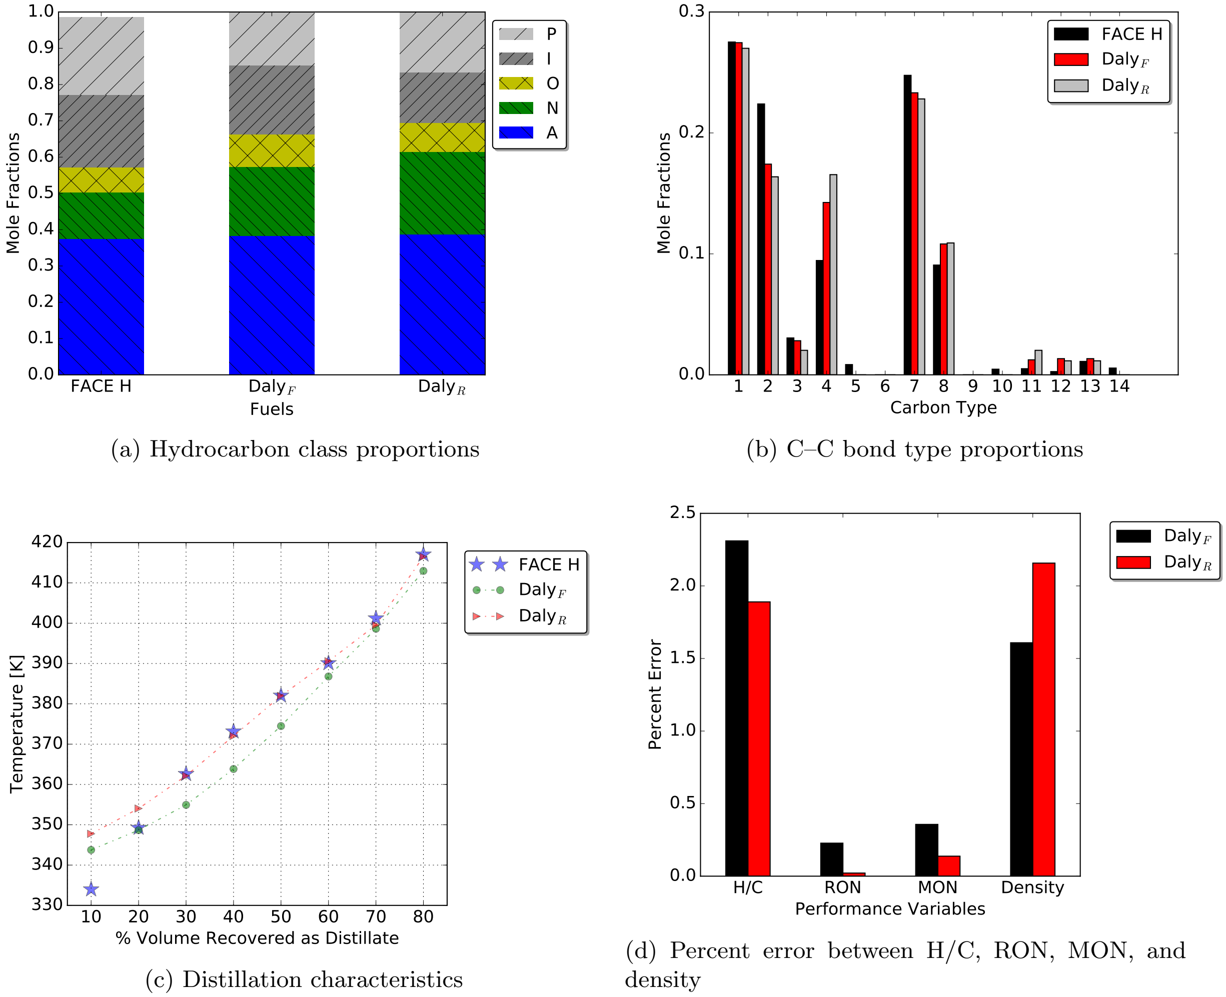


(a) Hydrocarbon class proportions

(b) C–C bond type proportions

(c) Distillation characteristics

(d) Percent error between H/C, RON, MON, and density

Figure 8: Target property comparisons for FACE H and surrogates developed in this work.

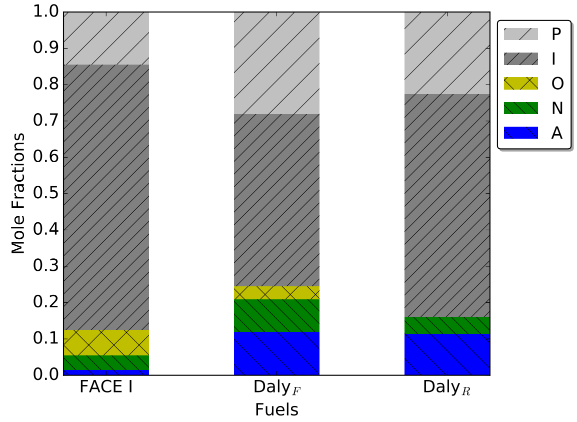


(a) Hydrocarbon class proportions

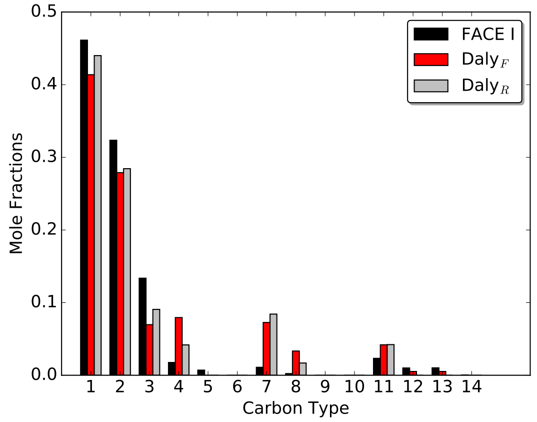


(b) C–C bond type proportions

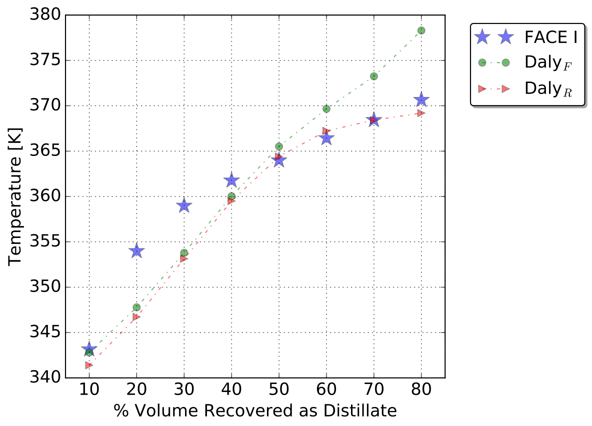


(c) Distillation characteristics

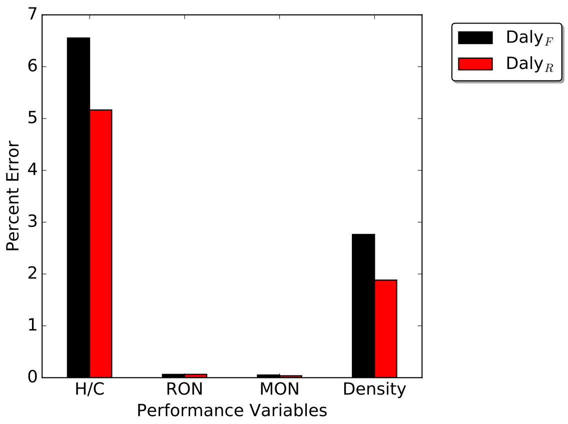


(d) Percent error between H/C, RON, MON, and density

Figure 9: Target property comparisons for FACE I and surrogates developed in this work.

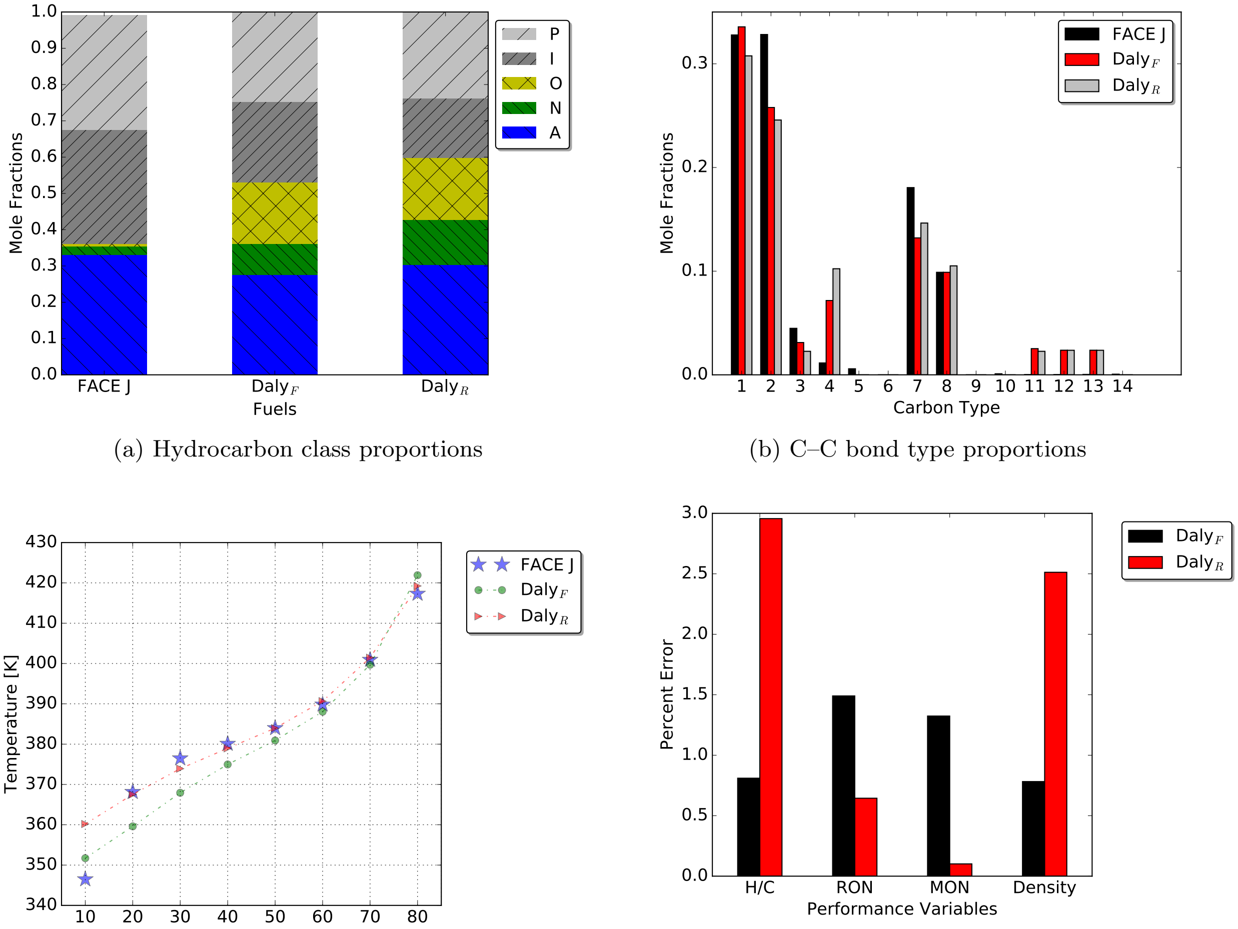


(a) Hydrocarbon class proportions

(b) C–C bond type proportions

(c) Distillation characteristics

(d) Percent error between H/C, RON, MON, and density

Figure 10: Target property comparisons for FACE J and surrogates developed in this work.
